# Supplementary material for: Relativistic and electron-correlation effects in static dipole polarizabilities for group 12 elements
Source: arXiv:2411.05394 source file (2025-01-17)
Supplement: Supplementary file 1 [file si.pdf]

# Supplemental Material for “Relativistic and electron-correlation effects in static dipole polarizabilities for group 12 elements”

YingXing Cheng\*

*Institute of Applied Analysis and Numerical Simulation, University of Stuttgart,  
Pfaffenwaldring 57, 70569, Stuttgart, Germany*

E-mail: [yingxing.cheng@mathematik.uni-stuttgart.de](mailto:yingxing.cheng@mathematik.uni-stuttgart.de)

## Contents

|                                                        |    |
|--------------------------------------------------------|----|
| S1 Hyperpolarizabilities Derived from Fitting Eq. (S1) | 3  |
| S2 Polarizabilities Derived from Fitting Eq. (S2)      | 6  |
| References                                             | 10 |

Static dipole polarizabilities ( $\alpha$ ) and hyperpolarizabilities ( $\gamma$ ) are determined using the finite-field method 1. The energy of an atom placed in an external electric field of magnitude  $F_z$  along the  $z$  axis is expressed as

$$E(F_z) \approx E_0 - \frac{1}{2}\alpha F_z^2 - \frac{1}{24}\gamma F_z^4, \quad (\text{S1})$$

where  $E_0$  represents the energy of the atom in the absence of the field. By applying least-squares fitting to energies computed at various field strengths, values for  $\alpha$  and  $\gamma$  were extracted. If  $\gamma$  yielded unphysical results, only  $\alpha$  was retained using the simplified expression

$$E(F_z) \approx E_0 - \frac{1}{2}\alpha F_z^2. \quad (\text{S2})$$

Each calculation is identified using a string representation of the computational setup, such as “2C-SR-CC@s-aug-ANO-RCC@(core 3)[vir 279]”. These identifiers consist of components separated by the delimiter “@”:

1. The first part specifies the computational method (e.g., NR-CC, SR-CC, or DC-CC), with the prefix “1C” or “2C” indicating the use of one- or two-component relativistic Hamiltonians, respectively.
2. The second part denotes the basis set.
3. The third part describes the correlation level, providing details on the number of active electrons and virtual orbitals as “(core  $N$ )[vir  $M$ ]. Here, “ $N$ ” is the total number of valence and outer-core electrons, and “ $M$ ” specifies the virtual orbitals included. The coupled-cluster module 2 supports a variety of correlated methods, including DHF, MP2, CCSD, and CCSD(T), all adhering to this identifier format.

Additional details can be found in the main text.

The percentage error  $\delta_m$  of a property  $X = \alpha$  or  $\gamma$  is computed as

$$\delta_m = \frac{X_m - X_{\text{CCSD(T)}}}{X_{\text{CCSD(T)}}} \times 100\%, \quad (\text{S3})$$

where  $m$  refers to the method employed, such as DHF, MP2, or CCSD. For  $X = \gamma$ ,  $\gamma_{\text{CCSD}}$  is used as the reference in Eq. (S3) instead of  $\gamma_{\text{CCSD(T)}}$ .

## S1 Hyperpolarizabilities Derived from Fitting Eq. (S1)

Table S1 presents the  $\gamma$  values for group 12 elements obtained by fitting Eq. (S1). For clarity, all negative  $\gamma$  values have been excluded from the table.

Table S1: Dipole hyperpolarizabilities ( $\gamma$ , in  $10^4$  a.u.) for group 12 elements. Uncertainties due to the numerical fitting procedure ( $\Delta P_{\text{fitting}}$ ) are shown as error bars for values exceeding 500 a.u.

| <b>Z</b> | <b>Atom</b> | <b><math>\gamma</math> (<math>10^4</math> a.u.)</b> | <b><math>\delta</math> (%)</b> | <b>Method</b> | <b>Comments</b>                              |
|----------|-------------|-----------------------------------------------------|--------------------------------|---------------|----------------------------------------------|
| 30       | Zn          | $54.16 \pm 0.01$                                    | 33.67                          | DHF           | 1C-NR-CC@s-aug-dyall.cv4z@(core 20)[vir 276] |
|          |             | 37.22                                               | -8.14                          | MP2           |                                              |
|          |             | 42.05                                               | 3.77                           | CCSD          |                                              |
|          |             | 40.52                                               | —                              | CCSD(T)       |                                              |
|          |             | 50.83                                               | 35.48                          | DHF           | 1C-SR-CC@dyall.cv4z@(core 20)[vir 204]       |
|          |             | 33.76                                               | -10.01                         | MP2           |                                              |
|          |             | 39.00                                               | 3.96                           | CCSD          |                                              |
|          |             | 37.52                                               | —                              | CCSD(T)       |                                              |
|          |             | $50.93 \pm 0.01$                                    | 33.91                          | DHF           | 1C-SR-CC@s-aug-dyall.cv4z@(core 20)[vir 276] |
|          |             | 34.65                                               | -8.90                          | MP2           |                                              |
|          |             | 39.48                                               | 3.79                           | CCSD          |                                              |
|          |             | 38.04                                               | —                              | CCSD(T)       |                                              |
|          |             | $50.95 \pm 0.01$                                    | 33.94                          | DHF           | 1C-SR-CC@d-aug-dyall.cv4z@(core 20)[vir 348] |
|          |             | 34.71                                               | -8.77                          | MP2           |                                              |
|          |             | 39.49                                               | 3.80                           | CCSD          |                                              |
|          |             | 38.04                                               | —                              | CCSD(T)       |                                              |
|          |             | $50.92 \pm 0.01$                                    | 33.61                          | DHF           | 2C-DC-CC@s-aug-ANO-RCC@(core 20)[vir 314]    |
|          |             | 34.72                                               | -8.88                          | MP2           |                                              |
|          |             | 39.60                                               | 3.91                           | CCSD          |                                              |

(continued)

Table S1. continued.

| Z  | Atom | $\gamma$ ( $10^4$ a.u.) | $\delta$ | Method  | Comments                                     |
|----|------|-------------------------|----------|---------|----------------------------------------------|
| 48 | Cd   | 38.11                   | --       | CCSD(T) |                                              |
|    |      | $50.89 \pm 0.01$        | 33.92    | DHF     | 2C-DC-CC@s-aug-dyall.cv4z@(core 20)[vir 276] |
|    |      | 34.62                   | -8.91    | MP2     |                                              |
|    |      | 39.44                   | 3.79     | CCSD    |                                              |
|    |      | 38.00                   | --       | CCSD(T) |                                              |
|    |      | $76.25 \pm 0.02$        | 40.26    | DHF     | 1C-NR-CC@s-aug-dyall.cv4z@(core 30)[vir 344] |
|    |      | 44.86                   | -17.48   | MP2     |                                              |
|    |      | $57.26 \pm 0.01$        | 5.32     | CCSD    |                                              |
|    |      | $54.36 \pm 0.01$        | --       | CCSD(T) |                                              |
|    |      | $63.82 \pm 0.01$        | 39.91    | DHF     | 1C-SR-CC@dyall.cv4z@(core 30)[vir 272]       |
|    |      | 36.70                   | -19.55   | MP2     |                                              |
|    |      | 47.97                   | 5.16     | CCSD    |                                              |
|    |      | 45.62                   | --       | CCSD(T) |                                              |
|    |      | $63.95 \pm 0.01$        | 39.50    | DHF     | 1C-SR-CC@s-aug-dyall.cv4z@(core 30)[vir 344] |
|    |      | 37.22                   | -18.79   | MP2     |                                              |
|    |      | $48.17 \pm 0.01$        | 5.09     | CCSD    |                                              |
|    |      | $45.84 \pm 0.01$        | --       | CCSD(T) |                                              |
| 80 | Hg   | $63.95 \pm 0.01$        | 39.49    | DHF     | 1C-SR-CC@d-aug-dyall.cv4z@(core 30)[vir 416] |
|    |      | 37.24                   | -18.77   | MP2     |                                              |
|    |      | $48.18 \pm 0.01$        | 5.09     | CCSD    |                                              |
|    |      | $45.84 \pm 0.01$        | --       | CCSD(T) |                                              |
|    |      | $63.75 \pm 0.01$        | 39.70    | DHF     | 2C-DC-CC@s-aug-ANO-RCC@(core 30)[vir 366]    |
|    |      | 38.11                   | -16.48   | MP2     |                                              |
|    |      | $47.68 \pm 0.01$        | 4.48     | CCSD    |                                              |
|    |      | $45.63 \pm 0.01$        | --       | CCSD(T) |                                              |
|    |      | $63.83 \pm 0.01$        | 39.51    | DHF     | 2C-DC-CC@s-aug-dyall.cv4z@(core 30)[vir 344] |
|    |      | 37.16                   | -18.79   | MP2     |                                              |
|    |      | $48.09 \pm 0.01$        | 5.10     | CCSD    |                                              |
|    |      | $45.75 \pm 0.01$        | --       | CCSD(T) |                                              |
|    |      | $81.65 \pm 0.02$        | 43.27    | DHF     | 1C-NR-CC@s-aug-dyall.cv4z@(core 44)[vir 362] |
|    |      | $44.25 \pm 0.01$        | -22.36   | MP2     |                                              |
|    |      | $60.33 \pm 0.01$        | 5.86     | CCSD    |                                              |
|    |      | $56.99 \pm 0.01$        | --       | CCSD(T) |                                              |
|    |      | 45.12                   | 32.32    | DHF     | 1C-SR-CC@dyall.cv4z@(core 44)[vir 290]       |
|    |      | 27.21                   | -20.19   | MP2     |                                              |
|    |      | 35.34                   | 3.64     | CCSD    |                                              |
|    |      | 34.10                   | --       | CCSD(T) |                                              |
|    |      | $45.20 \pm 0.01$        | 31.99    | DHF     | 1C-SR-CC@s-aug-dyall.cv4z@(core 44)[vir 362] |
|    |      |                         |          |         |                                              |
|    |      |                         |          |         |                                              |

(continued)

Table S1. continued.

| Z | Atom | $\gamma$ ( $10^4$ a.u.) | $\delta$ | Method  | Comments                                     |
|---|------|-------------------------|----------|---------|----------------------------------------------|
|   |      | 27.47                   | -19.79   | MP2     |                                              |
|   |      | 35.47                   | 3.57     | CCSD    |                                              |
|   |      | 34.25                   | --       | CCSD(T) |                                              |
|   |      | 45.20 $\pm$ 0.01        | 32.25    | DHF     | 1C-SR-CC@d-aug-dyall.cv4z@(core 44)[vir 460] |
|   |      | 27.35                   | -19.97   | MP2     |                                              |
|   |      | 35.42                   | 3.62     | CCSD    |                                              |
|   |      | 34.18                   | --       | CCSD(T) |                                              |
|   |      | 44.88 $\pm$ 0.01        | 30.52    | DHF     | 2C-DC-CC@s-aug-ANO-RCC@(core 44)[vir 282]    |
|   |      | 28.05                   | -18.43   | MP2     |                                              |
|   |      | 35.52                   | 3.30     | CCSD    |                                              |
|   |      | 34.39                   | --       | CCSD(T) |                                              |
|   |      | 44.94                   | 31.90    | DHF     | 2C-DC-CC@s-aug-dyall.cv4z@(core 44)[vir 362] |
|   |      | 27.38                   | -19.66   | MP2     |                                              |
|   |      | 35.29                   | 3.56     | CCSD    |                                              |
|   |      | 34.07                   | --       | CCSD(T) |                                              |
|   | 112  | 109.43 $\pm$ 0.04       | 47.38    | DHF     | 1C-NR-CC@s-aug-dyall.cv4z@(core 44)[vir 434] |
|   |      | 52.78 $\pm$ 0.01        | -28.92   | MP2     |                                              |
|   |      | 79.78 $\pm$ 0.02        | 7.45     | CCSD    |                                              |
|   |      | 74.25 $\pm$ 0.02        | --       | CCSD(T) |                                              |
|   |      | 30.25                   | 8.87     | DHF     | 1C-SR-CC@dyall.cv4z@(core 44)[vir 336]       |
|   |      | 25.83                   | -7.06    | MP2     |                                              |
|   |      | 27.81                   | 0.10     | CCSD    |                                              |
|   |      | 27.79                   | --       | CCSD(T) |                                              |
|   |      | 30.26                   | 9.09     | DHF     | 1C-SR-CC@s-aug-dyall.cv4z@(core 44)[vir 434] |
|   |      | 25.79                   | -7.02    | MP2     |                                              |
|   |      | 27.77                   | 0.12     | CCSD    |                                              |
|   |      | 27.73                   | --       | CCSD(T) |                                              |
|   |      | 30.26                   | 9.12     | DHF     | 1C-SR-CC@d-aug-dyall.cv4z@(core 44)[vir 532] |
|   |      | 25.75                   | -7.11    | MP2     |                                              |
|   |      | 27.76                   | 0.13     | CCSD    |                                              |
|   |      | 27.73                   | --       | CCSD(T) |                                              |
|   |      | 30.52                   | 8.71     | DHF     | 4C-DC-CC@dyall.cv4z@(core 12)[vir 264]       |
|   |      | 26.93                   | -4.08    | MP2     |                                              |
|   |      | 27.98                   | -0.33    | CCSD    |                                              |
|   |      | 28.07                   | --       | CCSD(T) |                                              |
|   |      | 30.47                   | 9.11     | DHF     | 2C-DC-CC@s-aug-dyall.cv4z@(core 48)[vir 434] |
|   |      | 25.97                   | -7.01    | MP2     |                                              |
|   |      | 27.95                   | 0.08     | CCSD    |                                              |

(continued)

Table S1. continued.

| <b>Z</b> | <b>Atom</b> | <b><math>\gamma</math> (<math>10^4</math> a.u.)</b> | <b><math>\delta</math></b> | <b>Method</b> | <b>Comments</b> |
|----------|-------------|-----------------------------------------------------|----------------------------|---------------|-----------------|
|          |             | 27.93                                               | --                         | CCSD(T)       |                 |

A summary of the highlighted  $\gamma$  values for group 12 elements is provided in Table S2, based on data from Table S1.

Table S2: Static hyperpolarizabilities (in  $10^4$  a.u.) with nonrelativistic, scalar-relativistic, full Dirac-Coulomb relativistic effects of group 12 elements.

| $\hat{H}$ | Method  | Zn              | Cd               | Hg               | Cn               |
|-----------|---------|-----------------|------------------|------------------|------------------|
| NR        | DHF     | $4.54 \pm 0.33$ | $11.58 \pm 0.14$ | $11.21 \pm 0.17$ | $21.62 \pm 0.23$ |
|           | CCSD    | $2.63 \pm 0.33$ | $6.64 \pm 0.14$  | $6.79 \pm 0.17$  | $12.86 \pm 0.23$ |
|           | CCSD(T) | $2.40 \pm 0.43$ | $5.90 \pm 0.14$  | $6.06 \pm 0.28$  | $11.32 \pm 0.34$ |
| SR        | DHF     | 4.48            | 8.07             | 3.16             | 0.57             |
|           | CCSD    | 2.61            | 4.44             | 1.99             | -0.49            |
|           | CCSD(T) | $2.39 \pm 0.19$ | $3.88 \pm 0.06$  | $1.81 \pm 0.22$  | $-0.71 \pm 0.54$ |
| DC        | DHF     | 4.49            | 8.01             | 3.04             | 0.51             |
|           | CCSD    | 2.59            | 4.41             | 2.00             | -0.43            |
|           | CCSD(T) | $2.38 \pm 0.19$ | 3.86             | $1.81 \pm 0.21$  | $-0.65 \pm 1.18$ |

## S2 Polarizabilities Derived from Fitting Eq. (S2)

Table S3 lists the  $\alpha$  values for group 12 elements, obtained using Eq. (S2). The most accurate results for NR-CC, SR-CC, and DC-CC calculations are highlighted.

Table S3: Dipole polarizabilities ( $\alpha$ , in a.u.) for group 12 elements. Error bars reflect the uncertainties arising from the numerical fitting procedure ( $\Delta P_{\text{fitting}}$ ) for cases where the errors exceed 0.005 a.u.

| <b>Z</b> | <b>Atom</b> | <b><math>\alpha</math> (a.u.)</b> | <b><math>\delta</math> (%)</b> | <b>Method</b> | <b>Comments</b>                              |
|----------|-------------|-----------------------------------|--------------------------------|---------------|----------------------------------------------|
| 30       | Zn          | $54.07 \pm 0.01$                  | 33.60                          | DHF           | 1C-NR-CC@s-aug-dyall.cv4z@(core 20)[vir 276] |
|          |             | $37.18 \pm 0.01$                  | -8.13                          | MP2           |                                              |
|          |             | $41.99 \pm 0.01$                  | 3.76                           | CCSD          |                                              |
|          |             | $40.47 \pm 0.01$                  | --                             | CCSD(T)       |                                              |
|          |             | 50.79                             | 35.46                          | DHF           | 1C-SR-CC@dyall.cv4z@(core 20)[vir 204]       |

(continued)

Table S3. continued.

| Z | Atom | $\alpha$ (a.u.) | $\delta$ | Method  | Comments |
|---|------|-----------------|----------|---------|----------|
|   |      | 33.74           | -10.02   | MP2     |          |
|   |      | 38.98           | 3.96     | CCSD    |          |
|   |      | 37.49           | --       | CCSD(T) |          |
|   |      | 50.84           | 33.84    | DHF     |          |
|   |      | 34.61           | -8.89    | MP2     |          |
|   |      | 39.43           | 3.79     | CCSD    |          |
|   |      | 37.99           | --       | CCSD(T) |          |
|   |      | 50.84           | 33.84    | DHF     |          |
|   |      | 34.67           | -8.73    | MP2     |          |
|   |      | 39.43           | 3.79     | CCSD    |          |
|   |      | 37.99           | --       | CCSD(T) |          |
|   |      | 50.81           | 33.51    | DHF     |          |
|   |      | 34.69           | -8.85    | MP2     |          |
|   |      | 39.54           | 3.90     | CCSD    |          |
|   |      | 38.06           | --       | CCSD(T) |          |
|   |      | 50.80           | 33.85    | DHF     |          |
|   |      | 34.57           | -8.90    | MP2     |          |
|   |      | 39.39           | 3.79     | CCSD    |          |
|   |      | 37.95           | --       | CCSD(T) |          |
|   |      | 76.02           | 40.14    | DHF     |          |
|   |      | 44.80           | -17.41   | MP2     |          |
|   |      | 57.12           | 5.31     | CCSD    |          |
|   |      | 54.24           | --       | CCSD(T) |          |
|   |      | 63.76           | 39.90    | DHF     |          |
|   |      | 36.65           | -19.58   | MP2     |          |
|   |      | 47.92           | 5.16     | CCSD    |          |
|   |      | 45.57           | --       | CCSD(T) |          |
|   |      | 63.78           | 39.38    | DHF     |          |
|   |      | 37.19           | -18.72   | MP2     |          |
|   |      | 48.08           | 5.08     | CCSD    |          |
|   |      | 45.76           | --       | CCSD(T) |          |
|   |      | 63.78           | 39.37    | DHF     |          |
|   |      | 37.21           | -18.69   | MP2     |          |
|   |      | 48.09           | 5.08     | CCSD    |          |
|   |      | 45.76           | --       | CCSD(T) |          |
|   |      | 63.59           | 39.59    | DHF     |          |
|   |      | 38.08           | -16.40   | MP2     |          |
|   |      | 47.59           | 4.47     | CCSD    |          |

(continued)

Table S3. continued.

| Z   | Atom | $\alpha$ (a.u.)  | $\delta$ | Method  | Comments                                     |
|-----|------|------------------|----------|---------|----------------------------------------------|
| 80  | Hg   | 45.55            | --       | CCSD(T) |                                              |
|     |      | 63.67            | 39.39    | DHF     | 2C-DC-CC@s-aug-dyall.cv4z@(core 30)[vir 344] |
|     |      | 37.12            | -18.72   | MP2     |                                              |
|     |      | 48.00            | 5.08     | CCSD    |                                              |
|     |      | 45.68            | --       | CCSD(T) |                                              |
|     |      | 81.43            | 43.18    | DHF     | 1C-NR-CC@s-aug-dyall.cv4z@(core 44)[vir 362] |
|     |      | 44.17            | -22.33   | MP2     |                                              |
|     |      | 60.19 $\pm$ 0.01 | 5.84     | CCSD    |                                              |
|     |      | 56.87 $\pm$ 0.01 | --       | CCSD(T) |                                              |
|     |      | 45.08            | 32.30    | DHF     | 1C-SR-CC@dyall.cv4z@(core 44)[vir 290]       |
|     |      | 27.20            | -20.18   | MP2     |                                              |
|     |      | 35.32            | 3.64     | CCSD    |                                              |
|     |      | 34.08            | --       | CCSD(T) |                                              |
|     |      | 45.14            | 31.94    | DHF     | 1C-SR-CC@s-aug-dyall.cv4z@(core 44)[vir 362] |
|     |      | 27.46            | -19.72   | MP2     |                                              |
|     |      | 35.43            | 3.56     | CCSD    |                                              |
|     |      | 34.21            | --       | CCSD(T) |                                              |
|     |      | 45.14            | 32.21    | DHF     | 1C-SR-CC@d-aug-dyall.cv4z@(core 44)[vir 460] |
|     |      | 27.35            | -19.88   | MP2     |                                              |
|     |      | 35.37 $\pm$ 0.01 | 3.61     | CCSD    |                                              |
|     |      | 34.14 $\pm$ 0.01 | --       | CCSD(T) |                                              |
|     |      | 44.82            | 30.50    | DHF     | 2C-DC-CC@s-aug-ANO-RCC@(core 44)[vir 282]    |
|     |      | 28.04            | -18.34   | MP2     |                                              |
|     |      | 35.47 $\pm$ 0.01 | 3.29     | CCSD    |                                              |
|     |      | 34.34 $\pm$ 0.01 | --       | CCSD(T) |                                              |
|     |      | 44.88            | 31.86    | DHF     | 2C-DC-CC@s-aug-dyall.cv4z@(core 44)[vir 362] |
|     |      | 27.37            | -19.59   | MP2     |                                              |
|     |      | 35.25            | 3.56     | CCSD    |                                              |
|     |      | 34.04            | --       | CCSD(T) |                                              |
| 112 | Cn   | 108.99           | 47.24    | DHF     | 1C-NR-CC@s-aug-dyall.cv4z@(core 44)[vir 434] |
|     |      | 52.65            | -28.87   | MP2     |                                              |
|     |      | 79.52 $\pm$ 0.01 | 7.43     | CCSD    |                                              |
|     |      | 74.02 $\pm$ 0.01 | --       | CCSD(T) |                                              |
|     |      | 30.24            | 8.78     | DHF     | 1C-SR-CC@dyall.cv4z@(core 44)[vir 336]       |
|     |      | 25.82            | -7.13    | MP2     |                                              |
|     |      | 27.83 $\pm$ 0.01 | 0.09     | CCSD    |                                              |
|     |      | 27.80 $\pm$ 0.01 | --       | CCSD(T) |                                              |
|     |      | 30.24            | 8.99     | DHF     | 1C-SR-CC@s-aug-dyall.cv4z@(core 44)[vir 434] |
|     |      |                  |          |         |                                              |

(continued)



Table S3. continued.

| Z | Atom | $\alpha$ (a.u.)  | $\delta$ | Method  | Comments                                     |
|---|------|------------------|----------|---------|----------------------------------------------|
|   |      | 25.78            | -7.09    | MP2     |                                              |
|   |      | $27.78 \pm 0.01$ | 0.11     | CCSD    |                                              |
|   |      | $27.75 \pm 0.01$ | --       | CCSD(T) |                                              |
|   |      | 30.25            | 9.04     | DHF     | 1C-SR-CC@d-aug-dyall.cv4z@(core 44)[vir 532] |
|   |      | 25.75            | -7.17    | MP2     |                                              |
|   |      | $27.77 \pm 0.01$ | 0.12     | CCSD    |                                              |
|   |      | $27.74 \pm 0.01$ | --       | CCSD(T) |                                              |
|   |      | 30.51            | 8.71     | DHF     | 4C-DC-CC@dyall.cv4z@(core 12)[vir 264]       |
|   |      | 26.92            | -4.07    | MP2     |                                              |
|   |      | 27.97            | -0.33    | CCSD    |                                              |
|   |      | 28.07            | --       | CCSD(T) |                                              |
|   |      | 30.46            | 9.01     | DHF     | 2C-DC-CC@s-aug-dyall.cv4z@(core 48)[vir 434] |
|   |      | 25.97            | -7.08    | MP2     |                                              |
|   |      | $27.96 \pm 0.02$ | 0.06     | CCSD    |                                              |
|   |      | $27.94 \pm 0.02$ | --       | CCSD(T) |                                              |

Table S4 summarizes the most accurate  $\alpha$  results for group 12 elements, as derived from Table S3.

Table S4: Static dipole polarizabilities (in a.u.) are presented with nonrelativistic, scalar-relativistic, and fully relativistic Dirac-Coulomb contributions for the elements of group 12, compared with the values reported in Ref. 3. The uncertainty due to the numerical fitting procedure ( $\Delta P_{\text{fitting}}$ ) is accounted for as the error bar. Only uncertainties where  $\Delta P_{\text{fitting}} > 0.005$  a.u. are shown.

| $\hat{H}$ | Method  | Zn               | Cd               | Hg               | Cn                |
|-----------|---------|------------------|------------------|------------------|-------------------|
| NR        | DHF     | $54.16 \pm 0.01$ | $76.25 \pm 0.02$ | $81.65 \pm 0.02$ | $109.43 \pm 0.04$ |
|           | CCSD    | $42.05 \pm 0.01$ | $57.26 \pm 0.02$ | $60.33 \pm 0.02$ | $79.78 \pm 0.04$  |
|           | CCSD(T) | 40.52            | $54.36 \pm 0.01$ | $56.99 \pm 0.01$ | $74.25 \pm 0.02$  |
| SR        | DHF     | $50.93 \pm 0.01$ | $63.95 \pm 0.01$ | $45.20 \pm 0.01$ | 30.26             |
|           | CCSD    | $39.48 \pm 0.01$ | $48.17 \pm 0.01$ | $35.47 \pm 0.01$ | 27.77             |
|           | CCSD(T) | 38.04            | $45.84 \pm 0.01$ | 34.25            | 27.73             |
| DC        | DHF     | $50.89 \pm 0.01$ | $63.83 \pm 0.01$ | 44.94            | 30.47             |
|           | CCSD    | $39.44 \pm 0.01$ | $48.09 \pm 0.01$ | 35.29            | 27.95             |
|           | CCSD(T) | 38.00            | $45.75 \pm 0.01$ | 34.07            | 27.93             |
| Ref. 3    | --      | $38.67 \pm 0.3$  | $46 \pm 2$       | $33.91 \pm 0.34$ | $28 \pm 2$        |

## References

- (1) Das, A. K.; Thakkar, A. J. Static Response Properties of Second-Period Atoms: Coupled Cluster Calculations. *J. Phys. B At. Mol. Opt. Phys.* **1998**, *31*, 2215.
- (2) DIRAC18. <https://doi.org/10.5281/zenodo.2253986>, Accessed on Jun 7, 2021.
- (3) Schwerdtfeger, P.; Nagle, J. K. 2018 Table of Static Dipole Polarizabilities of the Neutral Elements in the Periodic Table. *Mol. Phys.* **2019**, *117*, 1200–1225.
